# Supplementary material for: Topological properties of basins of attraction and expressiveness of width bounded neural networks
Source: arXiv:2011.04923 ancillary file (2023-12-01)
Supplement: Supplementary file 1 [file supplementary_material.pdf]

---

# Expressiveness of Neural Networks Having Width Equal or Below the Input Dimension

## Supplementary Material

---

**Hans-Peter Beise**

Department of Computer Science  
Trier University of Applied Sciences  
H.Beise@hochschule-trier.de

**Steve Dias Da Cruz**

IEE S.A.  
University of Kaiserslautern  
steve.dias-da-cruz@iee.lu

The following example shows that the maximum principle in Theorem 3 does not hold when the rank of the weight matrices is restricted to be equal or less the input dimension, but the width of the network function is allowed to be larger than the input dimension.

### Example 1

Let  $M = [-1, 1]$  and let  $W_1 \in \mathbb{R}^{2 \times 1}$  and  $b_1 \in \mathbb{R}^2$  implement the following linear affine mapping

$$W_1 x + b_1 = \begin{pmatrix} x + 1 \\ x \end{pmatrix}.$$

Then  $M_1 = \text{ReLU}(W_1 M + b_1)$  is given by  $M_1 = M_{1,1} \cup M_{1,2}$  where

$$M_{1,1} := \{(x + 1, 0)^T : x \in M, \text{ and } x < 0\}$$

$$M_{1,2} := \{(x + 1, x)^T : x^T \in M, \text{ and } x \geq 0\}.$$

Now, let  $v = (1, 1/2)^T \in \mathbb{R}^2$ ,  $W_2 \in \mathbb{R}^{2 \times 2}$  and  $b_2 \in \mathbb{R}^2$  such that  $x \mapsto W_2 x + b_2$  implements the orthogonal projection onto the hypersurface  $V := \{x \in \mathbb{R}^2 : x^T v = (1, 0)v\}$ . That is, the hypersurface orthogonal to  $v$  which intersects  $(1, 0)^T$ . Then both,  $M_{1,1}$  and  $M_{1,2}$  are mapped to the line  $M_2 := \{y \in \mathbb{R}^2 : y = (1, 0) + \lambda(-1/2, 1), 0 \leq \lambda \leq 1/2\}$  and since those vectors are contained in the first quadrant we have

$$M_2 = \text{ReLU}(W_2(\text{ReLU}(W_1 M + b_1) + b_1).$$

It can further easily be verified that, under the latter two layer network function, 0, which is an inner point of  $M$ , is the only vector that is mapped to the extreme point  $(1, 0)$  of  $M_2$ . Now it is easy to find a weight  $W_3 \in \mathbb{R}^2$  such that the linear map  $x \mapsto W_3 x$  as a mapping from  $M_2$  to  $\mathbb{R}$  takes its minimum or maximum value at  $(1, 0)$  only.

By concatenation of additional components to the input dimension such that  $M = [-1, 1] \times [0, 1]^d$ ,  $d \in \mathbb{N}$ , and adaptation of the weights  $W_1, W_2$  and bias  $b_1, b_2$  in a way that these additional components are mapped identically under the action of the two layer network function  $x \mapsto \text{ReLU}(W_2(\text{ReLU}(W_1 x + b_1) + b_1)$ , the above example can be extended to higher dimensions.

### Proof Proposition 1

*Proof.* We start with the proof of (1). It is clear that  $P_U$  followed by a linear isomorphism  $E : U \rightarrow \mathbb{R}^m$  with  $m = \dim(U) < n_0$  can be implemented by  $x \mapsto W_1 x + b_1$  with some  $W_1 \in \mathbb{R}^{m \times n_0}$ ,  $b_1 \in \mathbb{R}^m$ . As  $M$  is compact and hence bounded, one can further arrange  $b_1$  in a way that  $W_1 x + b_1 \geq 0$

holds (component wise) for every  $x \in M$ , which implies that  $\text{ReLU}(W_1x + b_1) = W_1x + b_1$  for all  $x \in M$ . Thus  $g(x) = \text{ReLU}(W_1x + b_1)$  maps  $M$  bijectively to  $M_1 := \text{ReLU}(W_1M + b_1) \subset \mathbb{R}^m$ . Now, uniform approximation of a given continuous function  $f$  from  $M$  to  $\mathbb{R}$  amounts to uniform approximation of continuous function from  $M_1$  to  $\mathbb{R}$ . By Tietze's Extension Theorem [?] we can apply Theorem 1 from [?] which yields arbitrary accurate uniform approximation of continuous function on rectangular domains in  $\mathbb{R}^m$  by network functions in  $\mathcal{NN}_{\text{ReLU}}(m+1)$ .

To show (2), let  $W_1 \in \mathbb{R}^{1 \times n_0}$  and  $b_1 \in \mathbb{R}$  such that  $y_j = W_1x_j + b_1$ ,  $j = 1, \dots, m$ , are distinct points  $M_1 = \{y_1, \dots, y_m\} \subset [0, \infty)$ . It is then clear that also  $F_0(x) := \text{ReLU}(W_1x + b_1)$  maps  $M$  to  $M_1$ . Now, for some function  $f : M \rightarrow \mathbb{R}$  (which is automatically continuous as  $M$  is finite) we have to find a network function  $F_1 \in \mathcal{NN}_{\text{ReLU}}(2)$  such that  $F_1(y_j) = f(x_j)$  for  $j = 1, \dots, m$ . To this end, we observe that the mapping  $y_j \mapsto f(x_j)$ ,  $j = 1, \dots, m$  can be interpolated by a max-min string, see [?], Definition 1] for a definition, so that [?, Proposition 2] yields the desired  $F_1$ . Alternatively, one could follow the proof of [?, Theorem 3.2.], observing that on the non-negative  $y_j$ ,  $j = 1, \dots, m$ , the residual ReLU network function constructed in the latter can be written as a ReLU network function in the sense of this work with width two in our case. Finally, we have that  $F = F_1 \circ F_0 \in \mathcal{NN}_{\text{ReLU}}(2)$  and  $F(x_j) = f(x_j)$  for all  $j = 1, \dots, m$ .  $\square$

## Proof Corollary 1

*Proof.* By means of Proposition 2, we find an  $F_1 \in \mathcal{NN}_{\text{ReLU}}^{n_0}(n_0)$  such that  $F_1(x) = x$  for  $x \in \bigcup_{j=2}^d K_j$  and  $a_1 := F_1(K_1)$  is a single vector in  $\mathbb{R}^{n_0} \setminus \bigcup_{j=2}^d K_j$ . Proposition 2 also allows us to choose  $F_1$  in a way that  $a_1$  is sufficiently close to  $K_1$  that the conditions of Theorem 1 still apply to  $\bigcup_{j=2}^d K_j \cup \{a_1\}$ . We can iteratively apply Proposition 2 to find  $F_1, \dots, F_d \in \mathcal{NN}_{\text{ReLU}}^{n_0}(n_0)$  such that

$$F_d \circ \dots \circ F_1(K_j) = a_j, \quad j = 1, \dots, d$$

for pairwise distinct  $a_1, \dots, a_d \in \mathbb{R}^{n_0}$ . Now, for a given  $f : M \rightarrow \mathbb{R}$  with  $f(x) = y_j$  for all  $x \in K_j$ ,  $j = 1, \dots, d$ , Proposition 1.2 yields an  $\tilde{F} \in \mathcal{NN}_{\text{ReLU}}(2)$  with  $\tilde{F}(a_j) = y_j$  for all  $j = 1, \dots, d$ . The desired network function is then obtained by  $F := \tilde{F} \circ F_d \circ \dots \circ F_1$ .  $\square$

## Proof Proposition 4

*Proof.* It is clear that the existence of inner points in  $F(M)$  requires that every weight matrix of  $F$  is square and of full rank. Indeed, otherwise the range of  $M$  is reduced to a manifold of dimension less than or equal to  $n_0 - 1$  after a layer that violates this condition. From then on the range remains without inner points. If  $L = 1$ , then we are done, since in this case  $F$  reduces to an isomorphism on  $\mathbb{R}^{n_0}$ . Otherwise, let  $M_j := A_j(M_{j-1})$  for  $j = 1, \dots, L$  and  $M_0 := M$ . Hence  $F(M) = M_L$ . Since  $W_L$  is non-singular,  $u_L \in M_L$  is an inner point of  $M_L$  if and only if  $u_L = W_L u_{L-1}$  for some unique point  $u_{L-1} \in M_{L-1}^\circ$ . This implies that component wise  $u_{L-1} > 0$  and further, by the fact that  $W_{L-1}$  is non-singular,  $u_{L-1} = W_{L-1} u_{L-2} + b_{L-1}$  for some unique point  $u_{L-2} \in M_{L-2}^\circ$ . The exact same reasoning can now iteratively be applied down to the first layer. This gives a sequence of  $u_j \in M_j^\circ$ ,  $j = 1, \dots, L$  so that component wise  $u_j > 0$  holds for every  $j$ . Hence,  $u_j = W_j u_{j-1} + b_j$  for  $j = 1, \dots, L$ . Thus, for the inverse image  $B = F^{-1}(F(M)^\circ) \subset M^\circ$ , the mapping  $F$  reduces to an bijective linear affine mapping.  $\square$

## Numerical Experiment

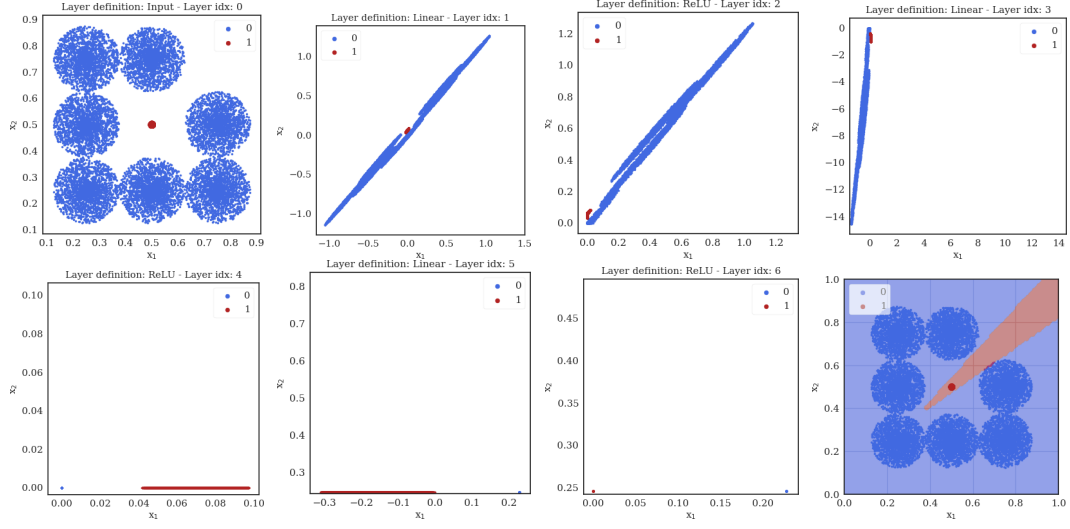

(a) 7 border balls - center ball radius: 0.01 - MSE: 0.0 - UUAC: 0.0

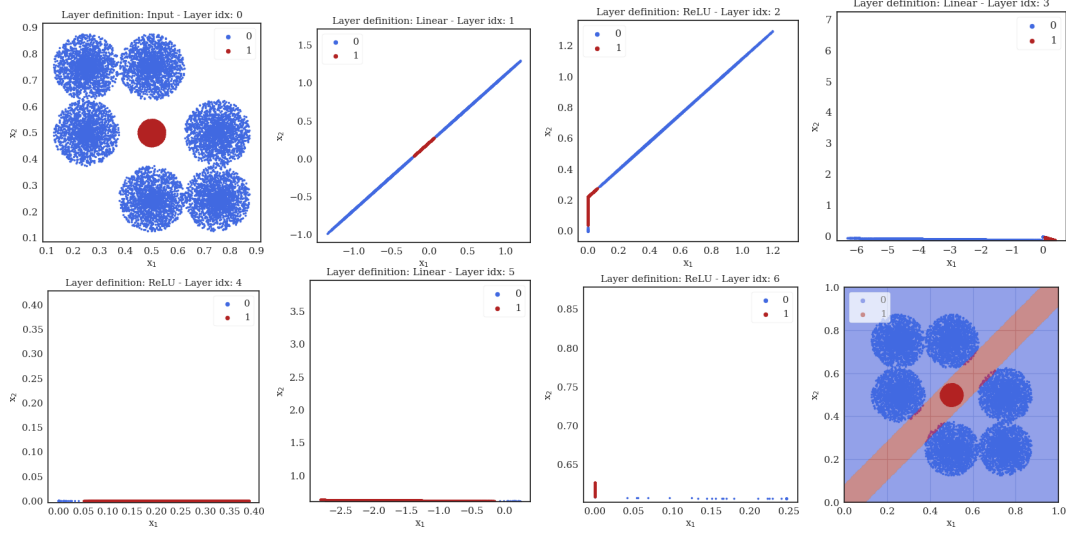

(b) 6 border balls - center ball radius: 0.05 - MSE: 0.00026 - UUAC: 0.99092

Figure 1: Additional results for Fig. 1 of the main paper. Different input datasets (a) and (b) together with the resulting transformations by each activation function and each layer learned by the neural network after 500 epochs. We also report the final decision regions, the mean-square error (MSE) and the universal uniform approximation condition (UUAC). When the conditions of Theorem 2 are fulfilled (a), the learned transformations are similar to the construction in the proof of Theorem 2. When the condition of Theorem is violated (b), the intermediate layers also violate the construction in the proof. The title of each subplot describes the function which is applied to the data of the previous subplot to form the data of the current subplot.
